# Supplementary material for: Enabling Deep Learning on Edge Devices
Source: arXiv:2210.03204 source file (2022-10-06)
Supplement: Supplementary file 1 [file A1_appendix.tex]

% !TEX root = 00_thesis.tex
%\appendix
%\chapter{Datasheets}
%%\section{Alpahsense NO2-B4 Nitrogen Dioxide Sensor 4-Electrode}
%\begin{figure}
%\centering
%\includegraphics[width=0.99\textwidth]{datasheets/NO2B4.pdf}
%\end{figure}
